# Supplementary material for: Fully Trainable and Interpretable Non-Local Sparse Models for Image Restoration
Source: arXiv:1912.02456 source file (2020-08-20)
Supplement: Supplementary file 2 [file supp_mat.tex]

\subsection{Proof of propostion \ref{csr_prox}}
The proximal operator of the function $\Psi_i(\ub) = \| \ub \|_1 + \gamma \| \ub - \betab_i \|_1$  for $\ub$ in~$\Real^p$ is defined as
\begin{equation*} \label{prox_psi}
    \prox_{\lambda \Psi_i} [\zb]=  \argmin_{\ub \in \Real^p} \frac{1}{2}\|\zb-\ub\|^2 + \lambda \|\ub\|_1 + \lambda \gamma \| \ub - \betab_i\|_1
\end{equation*}
The optimality condition for the previous problem is
$$ 0 \in \triangledown (\frac{1}{2} || \zb - \ub ||_2^2) + \partial (\lambda ||\ub||_1) + \partial (\lambda \gamma ||\ub - \betab_i||_1) $$
$$\Leftrightarrow 0 \in \ub - \zb + \lambda \partial ||\ub||_1 + \lambda \gamma  \partial ||\ub - \betab_i||_1  $$
We consider each component separately. We suppose that $\betab_i[j] \neq 0$, otherwise  $\Psi_i(\ub)[j]$ boils down to the $\ell_1$ norm. And we also suppose $\lambda,\gamma >0$.

Let's examine the first case where $u[j] = 0$. The subdifferential of the $\ell_1$ norm is the interval $[-1,1]$ and the optimality condition is
\begin{align*}
    0 \in \ub[j] - \zb[j] + [-\lambda,\lambda] + \lambda \gamma \sign(\ub[j]-\betab_i[j]) \\
    \Leftrightarrow \zb[j] \in [-\lambda,\lambda] -  \lambda \gamma \sign(\betab_i[j])
\end{align*}
Similarly if $\ub[j] = \betab_i[j]$
\begin{equation*}
    \zb[j] \in \betab_i[j] + \lambda \sign(\betab_i[j]) + [-\lambda \gamma,\lambda \gamma] 
\end{equation*}

Finally let's examine the case where $u[j] \neq 0$ and $u[j] \neq \betab_i[j]$: then, $\partial ||\ub||_1 = \sign(\ub[j])$ and $\partial ||\ub - \betab_i||_1 = \sign(\ub[j] - \betab_i[j])$. The minimum $u[j]^*$ is obtained as 
\begin{align*}
     0 = \ub[j] - \zb[j] + \lambda \sign(\ub[j]) + \lambda \gamma \sign(\ub[j]-\betab_i[j]) \\
     \Leftrightarrow \ub[j]^* =  \zb[j] - \lambda \sign(\ub[j]^*) - \lambda \gamma \sign(\ub[j]^*-\betab_i[j]) 
\end{align*}

We study separately the cases where $\ub[j]>\betab[j]$, $0<\ub[j]<\betab[j]$ and $\ub[j]<0$ when $\betab_i[j]>0$ and proceed similarly when $\betab_i<0$. With elementary operations we can derive the expression of $\zb[j]$ for each case. Putting the cases all together we obtain the formula.

\subsection{Additional experimental details}

In order to accelerate the inference time of the non-local models, we update patch similarities every $1/f$ steps. Where $f$ is the frequency of the correlation updates.
We summarize in Table \ref{hyperparam} the set of hyperparameters that we selected for the experiments reported in the main tables.
We selected the same hyper-parameters for the baselines, except that we do not compute pairwise patch similarities.

\begin{table}[h]
    \small
    \centering
    \caption{Hyper-parameters of our experiments.}
        \label{hyperparam}
    \begin{tabular}{lccc}
    \toprule
    Experiment & Color d. & Gray d. & Demosaicking \\
    \midrule
    Patch size & 7 & 9 & 9 \\
    Dictionnary size  &256 & 256 & 256 \\
    Nr epochs  & 300  &  300 & 200 \\
    Batch size &  25 & 25 & 16 \\
    $K$ iterations  & 24 & 24 & 24 \\
    \begin{tabular}[c]{@{}l@{}}Correlation update\\ frequency $f$\end{tabular} & ${1}/{6}$ & ${1}/{6}$ &  ${1}/{6}$ \\
    \bottomrule
    \end{tabular}

\end{table}

\subsection{Influence of patch and dictionnary size}

We investigate in Table \ref{ablation_table} the influence of two hyperparameters: the patch size and the dictionnary size for grayscale image denoising. For this experiment we run  a lighter version of the model groupSC, in order to accelerate the training. The batch size was decreased from 25 to 16, the frequency of the correlation updates was decreased from $1/6$ to $1/8$ and the intermediate patches are not approximated with averaging.  These changes accelerate the training but lead to slightly lower performances when compared with the model trained in the standard setting. It explains the gap between the scores in Table ~\ref{ablation_table} and in Table~\ref{gray_table}.

\begin{table}[h]
    \small
    \centering
    \caption{Influence of the dictionnary size and the patch size on the denoising performance. Grayscale denoising on BSD68. Models are trained on BSD400. Models are trained in a light setting to accelerate the training.}
    \label{ablation_table}
    \begin{tabular}{clccc}
        \toprule
        Noise ($\sigma$) &   Patch size   & n=128 & n=256 & 512   \\ 
        \midrule
        \multirow{3}{*}{$5$} 
        & k=7 &  37.91     &  37.92     & -     \\
        & k=9 &  37.90     & 37.92        &   37.96    \\
        & k=11 &  37.89     &  37.89      & -        \\
        \midrule
        \multirow{3}{*}{$15$} 
        & k=7 &   31.60    &  31.63       & -       \\
        & k=9 &   31.62    &31.67      & 31.71       \\
        & k=11 & 31.63  &  31.67      & -        \\
        \midrule
        \multirow{3}{*}{$25$}
        & k=7 &   29.10    & 29.11        & -       \\
        & k=9 &  29.12     & 29.17      &  29.20    \\
        & k=11 &  29.13     & 29.18      &-       \\
        \bottomrule
    \end{tabular}
\end{table}  

\subsection{Grayscale denoising: evaluation on multiple datasets}
We provide additional grayscale denoising results on other datasets in term of PSNR of our model in Table \ref{gray_app}.
\begin{table}[h]
\small
\centering
\caption{Grayscale denoising on different datasets.Training on BSD400.  Performance is measured in terms of average PSNR (in dB). }
\label{gray_app}
\begin{tabular}{cccccc}
    \toprule
    Dataset                   & Noise & BM3D  & DnCnn & NLRN  & {GroupSC} \\ 
    \midrule
    \multirow{4}{*}{\textbf{Set12}}   
        & 5    &  - &-&  -    &  38.40    \\
    & 15    & 32.37 & 32.86 & 33.16 & 32.85      \\
    & 25    & 29.97 & 30.44 & 30.80 &  30.44    \\
    & 50    & 26.72 & 27.18 & 27.64 &  27.14    \\
    \midrule
    \multirow{4}{*}{\textbf{BSD68}}    & 5  &  37.57&  37.68&  {37.92}     &  37.95    \\
    & 15    & 31.07 & 31.73 & 31.88 &   31.70   \\
    & 25    & 28.57 & 29.23 & 29.41 &   29.20   \\
    & 50    & 25.62 & 26.23 & 26.47 &  26.18    \\
    \midrule
    \multirow{4}{*}{\textbf{Urban100}}
    & 5     &   -    &    -  &    -   &  38.51    \\
    & 15    & 32.35 & 32.68 & 33.45 &   32.71   \\
    & 25    & 29.70 & 29.91 & 30.94 &  30.05    \\
    & 50    & 25.95 & 26.28 & 27.49 &  26.44  \\ \bottomrule
\end{tabular}
\end{table}

\subsection{Color denoising: evaluation on multiple datasets}
We provide additional color denoising results on other datasets in term of PSNR of our model in Table~\ref{color_app}.
\begin{table}[] 
    \small
    \centering
    \caption{Color denoising on different datasets.Training on CBSD400.  Performance is measured in terms of average PSNR (in dB). }
    \label{color_app}
    \begin{tabular}{cccc}
        \toprule 	
    Dataset                   & Noise& CBM3D & {GroupSC} \\ 	\midrule
    \multirow{4}{*}{\textbf{Kodak24}}   
    & 5   & -  &       40.72    \\
    & 15  &  33.25       &    34.98     \\
    & 25  &  32.06  &   32.44     \\
    &  50 &  28.75  &       29.16    \\
\midrule	\multirow{4}{*}{\textbf{CBSD68}}
    & 5  & 40.24  & 40.61     \\
    & 15 & 33.49  &  34.10    \\
    & 25 & 30.68 &  31.42    \\
    & 50 & 27.36 &  28.03   \\
\midrule	\multirow{4}{*}{\textbf{Urban100}} 
    &  5  & -         &  39.74 \\
    &  15  &    33.22     & 34.11  \\
    &  25  &   30.59     &  31.63   \\
    &  50  &   26.59     & 28.20    \\ 	\bottomrule
    \end{tabular}
\end{table}
